# Supplementary material for: FLAME: A Fast Large-scale Almost Matching Exactly Approach to Causal Inference
Source: arXiv:1707.06315 source file (2021-02-04)
Supplement: Supplementary file 1 [file algorithm-detail.tex]

% \section{FLAME Detailed Description}\label{sec:FLAMEPseudocode}

% \textcolor{red}{I stopped here.}

%Also, as FLAME successively drops covariates, it maintains a balance between treatment and control groups, in that when choosing which variable to eliminate at the next round, it considers the remaining fractions of treatment and control units, called the balancing factor, or $\BF$.

%For \BF, it is desirable that each dropped set of covariates maximizes the fraction of matched individuals from the available pools of units. If $\BF$ is high in earlier iterations, more of the matched units will exactly match on almost all covariates (in agreement with (R2)). We write this as follows (\#\ denotes `the number of'): 

%In matching, two basic requirements are 1) to match as many units as possible; and 2) match as exact (with respect to a certain metric). In our framework where the toenail problem are assumed to occur, we formalize the desiderata as: (\textbf{R1}) Each matched group contains at least one treatment unit (T = 1), and one control unit (T = 0). In addition, for a good matching quality, the following properties are desired: (\textbf{R2}) As many variables as possible $X^\prime$ from the set of covariates $X$ are used to define each group. (\textbf{R3}) The chosen covariates $X^\prime$ are sufficient to create a good predictor of potential outcome $Y$. (\textbf{R4}) As many units as possible from D should participate in the final matched groups. %(\textbf{R5}) (optional) The size of each group, and possibly the number of treated and control units, should be above a threshold.  
%To achieve a good balance of the properties listed above, we compute matched groups with subsets of variables. First, we match using all variables. The groups that have at least one treatment and one control unit are considered to be \emph{complete}, since we can directly estimate treatment effects for those groups, and the units are removed for the rest of the analysis. The remaining  groups will have either zero treatment or zero control units. If we do not continue trying to match we would violate (R4), but we must reduce the dimensionality of the space in order to match further. The idea of the framework is that when each unit is matched, it is matched on as many relevant dimensions as possible (R2), where relevant dimensions are those useful for prediction (R3). Matching with at least one treatment and one control (R1) is done for as many units as possible (R4). 

% The FLAME algorithm is a special case of the framework, where after the first level of exact matching when all identical units are removed, a second level of matching is done by omitting one variable from $X$, where the omitted variable is chosen based on optimization criteria for prediction quality (R3).  This process is repeated until either all units are matched or until we cannot remove variables without damaging prediction quality, so that (R3) would not be satisfied. Thus, the core of the algorithm is a scheme by which to sequentially reduce the number of variables that are being used to form exact matches without harming prediction quality. 
% \red{TODO for Alex: Please check your notes - anything else to add?} 

%A toy example using three variables is illustrated in  Figure~\ref{fig:FAMEillustration}. In this example a matching algorithm requires three steps and produces group labels $(E = e, G = g, H = h)$ describing education ($E$), gym membership ($G$), and home ownership ($H$) levels respectively. 
%\sudeepa{what should this be updated to?}\red{TODO: update this example} 
%First it considers all three variables and finds high quality exact matches. In this case the outcome of the first step is a collection of exactly-matched groups with labels  $\{(E = e, G = g, H = h):e\in\{No,HS\},g\in\{Y,N,M\},h\in\{Y,N\}\}$. The second step of the algorithm finds exact matches for the remaining individuals by considering only the gym and home variables. It constructs groups with labels $\{(\star, G = g, H = h):g=Y, h\in\{Y,N\}\}$ with $\star$ taking on any value in the domain of the corresponding variable (in this case $\{BA,MA,PhD\}$). Lastly, dropping the gym variable, exact matches are constructed using the home variable alone leading to group labels $\{(\star, \star, h): h\in\{Y,N\}\}$ where $\star$ again takes values in $\{BA,MA,PhD\}$ and $\triangle$ takes values in $\{N,M\}$. The first collection of matches is of the highest quality as it uses three variables, the second is of lower quality as it only uses two, and the last is of the lowest quality. This is in contrast to a coarsening approach \red{cite} that combines levels of covariates and then treats all matches as being of equal quality.


%\begin{figure}[tb]
%	\centering
%	\floatbox[{\capbeside\thisfloatsetup{capbesideposition={right,top},capbesidewidth=9.8cm}}]{figure}[\FBwidth]
%{	\caption{\sudeepa{do we need this figure and/or the example?} Illustrative example of an almost matching exactly algorithm. There are three variables (education: 5 levels, gym membership: 3 levels, and home ownership: 2 levels). There are exact matches for all three variables for levels ``No'' and ``HS'' of education (potentially 12 groups). There are exact matches for gym level yes and the home variable (potentially 2 groups). Finally there are exact matches based only on the home ownership variable.\label{fig:FAMEillustration}}}
%{	\includegraphics[scale=.3]{illustrative_example2.png}	}	\vspace{-0.75cm}
%\end{figure}
% \begin{algorithm}
%     \SetKwInOut{Input}{Input}
%     \SetKwInOut{Output}{Output}
%     \Input{Matching covariates $X$ (indexed by $J$), treatment indicator $T$, outcome variable $Y$.}
%     \Output{For each unit output a group label that describes the set of covariates that need to be used to maximize overall match quality.}

%     \For{lala}{haha}
%     \caption{Almost Exact Matching Algorithm}
% \end{algorithm}

%\subsection
