# Supplementary material for: FLAME: A Fast Large-scale Almost Matching Exactly Approach to Causal Inference
Source: arXiv:1707.06315 source file (2021-02-04)
Supplement: Supplementary file 2 [file experiments-detail.tex]

% \section{Experiments}

% \subsection{Variance estimation}

% \subsection{Experiments with Real Data}  %set from US Census 1990 Data:}
% %\textbf{Real dataset:} 

% \subsubsection{More Details on Prenatal Smoking on Infant's Abnormality} \label{exp:natality-detail2}

% Figure \ref{fig:natality-abnormal-2} serves as detailed supplements for Figure \ref{fig:natality-abnormal} in the main text.

% \begin{figure}[t]
% \centering
% %         \vspace{-2mm}
%      \caption{{\small In both subfigures, \textit{whole} on the x-axis corresponds to a plot for the whole population. 
% (a) 0: gestational hypertension is not reported; 1: is reported. 
% (b) 0: pregnancy diabetes is not reported; 1: is reported. 
% The presence of pregnancy diabetes or pregnancy hypertension leads to a higher variance in the treatment effect, and for diabetes, a higher treatment effect.
% }}
%      \vspace{-2mm}
%      \label{fig:natality-abnormal-2} 
% \end{figure}
