# Supplementary material for: FLAME: A Fast Large-scale Almost Matching Exactly Approach to Causal Inference
Source: arXiv:1707.06315 source file (2021-02-04)
Supplement: Supplementary file 3 [file proofs.tex]

% \section{Proofs and Additional Propositions}
% \label{app:proofs}

% \begin{proposition} 
% \label{thm:linear2} 
% Let $\mathcal{F} = \{f| f(\x) = \w^\top \x , \w \in \mathbb{R}^p \}$. Let $\{(x_i, y_i) \}_{i=1}^n$ be the holdout training dataset that is used to estimate $\hat{\PE_{\mathcal{F}}} (\btheta)$ for all $\btheta$. Then we have $\hat{\PE}_\mathcal{F} (\btheta) \ge \hat{\PE}_\mathcal{F} (\btheta^\prime)$ when $\btheta \le \btheta^\prime$ ($\le $ is the element-wise comparison operator for $\btheta$.). 
% %$\hat{\PE}_\mathcal{F} (\btheta) \le \hat{\PE}_\mathcal{F} (\btheta^\prime)$
% \end{proposition} 
% \begin{proof}
% \begin{align*}
%     \hat{\PE}_\mathcal{F} (\btheta) = \sum_{i=1}^n ( (\w_{\btheta} \circ \btheta)^\top (\x_i \circ \btheta) - y_i )^2 ,
% \end{align*} 
% where $\w_{\btheta} \in \arg \min_{\w} \sum_{i=1}^n ( (\w \circ \btheta)^\top (\x_i \circ \btheta) - y_i )^2 $. When  $\btheta^\prime \ge \btheta$, we can pick $\w^\prime$ such that it agrees with $\w_{\btheta}$ on the feature-selector $\btheta$'s covariates 
% %\textcolor{red}{ was this supposed to have a theta' in the equation? Where is theta'? } 
% $\w^\prime \circ \btheta = \w_{\btheta} \circ \btheta$, and is zero on other covariates, $\w^\prime \circ (\mathbf{1}_{p \times 1} - \btheta) = \mathbf{0}_{p \times 1}$. Then, since by our choice $\w^\prime \circ \btheta = \w_{\btheta} \circ \btheta$,
% $$\w^\prime \in \arg \min_{\w} \sum_{i=1}^n ( (\w \circ \btheta)^\top (\x_i \circ \btheta) - y_i )^2 .$$
% At the same time, $\w^\prime \circ \btheta^\prime = \w^\prime \circ \btheta$. Therefore
% \begin{align*}
%     &\quad \hat{\PE}_\mathcal{F} (\btheta) \\
%     &= \min_{\w} \sum_{i=1}^n ( (\w \circ \btheta)^\top (\x_i \circ \btheta) - y_i )^2 \\
%     &= \sum_{i=1}^n ( (\w_{\btheta} \circ \btheta)^\top (\x_i \circ \btheta) - y_i )^2 \\
%     &= \sum_{i=1}^n ( (\w^\prime \circ \btheta)^\top (\x_i \circ \btheta) - y_i )^2 \\
%     &=\sum_{i=1}^n ( (\w^\prime \circ \btheta^\prime)^\top (\x_i \circ \btheta^\prime) - y_i )^2 \\
%     &\ge \min_{\w} \sum_{i=1}^n ( (\w \circ \btheta^\prime)^\top (\x_i \circ \btheta^\prime) - y_i )^2 \\
%     &= \hat{\PE}_\mathcal{F} (\btheta^\prime).
% \end{align*}

% \end{proof}
