# Supplementary material for: FLAME: A Fast Large-scale Almost Matching Exactly Approach to Causal Inference
Source: arXiv:1707.06315 source file (2021-02-04)
Supplement: Supplementary file 4 [file sql.tex]

% \section{Database Implementation Details for BasicExactMatch}
% \label{app:sql}

% The pseudocode for subroutine \BasicExactMatch\ (for matching without replacement) used in Algorithm~\ref{algo:basic-FAME} appears in  Algorithm~\ref{algo:basicExactMatch}.
%  Below we discuss the implementation of \BasicExactMatch\ using SQL queries from databases, which was mentioned in Section~\ref{sec:algorithm-implementation}. An alternative implementation of \BasicExactMatch\ using bit-vectors is discussed in Section~\ref{sec:algorithm-implementation}.

%%%%%%%%%%%%%%%%%%%%%%%%%%%%%%% BasicExactMatch

% and let the treatment attribute $T$ be binary taking value 1 (for a treated observation) or 0 (for a control observation). 
%The SQL query is described in Appendix \ref{app:sql}. 
